# Supplementary material for: Towards a Dimension-Free Understanding of Adaptive Linear Control
Source: arXiv:2103.10620 source file (2021-07-15)
Supplement: Supplementary file 1 [file certainty_equivalence_app.tex]

%!TEX root = ../main.tex

\section{Proofs for Change of Measure}

\begin{theorem}
\label{theorem:HS_change_of_measure} 
Let $K_1 : \hilspace \to \R^{\dimu}$ be such that $A + B K_1$ is stable and let $\Lambda \in \psdhil$ be a trace class, positive semi-definite operator. Then, for any $K_2$ such that $A + BK_2$ is also stable, we have that
\begin{align*}
\dlyap{(A +BK_1)^\herm}{\Lambda} \preceq \dlyap{(A+ BK_2)^\herm}{\tLambda}
\end{align*}
where $\tLambda$ is a bounded operator  defined as
\begin{align*}
\tLambda \defeq 2\Lambda + 4 B (K_1 - K_2) \;\dlyapm{(A+BK_1)^\herm}{\Lambda}{2} \;(K_1 - K_2)^{\herm}B^{\herm}
\end{align*}
\end{theorem}

\begin{proof} We argue by constructing a hypothetical dynamical system and analyzing its behavior in two ways. In particular, define
\[	
\Aclone \defeq A + B K_1 \text{ and } \Acltwo \defeq A + B K_2
\]
and consider the system,
\begin{align}
\matx_{t+1} = \Aclone \matx_t + \matw_t, \text{ where }\matx_{0} = 0 \text { and } \forall \; t \ge 0, ~ \matw_t \iidsim \calN(0, \Lambda). \label{eq:first_system}
\end{align}
Then, for $\Sigma_1 \defeq \dlyap{\Aclone^\herm}{\Lambda}$ we have that
\begin{align*}
\Sigma_{1} =  \lim_{T \to \infty} \Sigma_{1;T}, \text{where } \Sigma_{1;T}  \defeq \Exp[\matx_T \otimes \matx_T],
\end{align*}
and where the above limit exists due to monotonicty of $\Sigma_{1;T}$. To prove our claim, let us express the evolution of \Cref{eq:first_system} as
\begin{align*}
\matx_{t+1} = \Acltwo \matx_t + (\Aclone - \Acltwo) \matx_t +  \matw_t = \Acltwo \matx_t + B \underbrace{(K_1 - K_2)\matx_t}_{:=\matu_t} + \matw_t.
\end{align*}

Define the deterministic operator
$G_{T} := \begin{bmatrix} I  \mid \Acltwo \mid \dots  \mid \Acltwo^{T-1}\end{bmatrix}: \hilspace^{T} \to \hilspace$, and the random vector
\begin{align*}
\matz_{[T]} := \begin{bmatrix} B \matu_{T-1} + \matw_{T-1} \\ \dots \\ B \matu_{1} + \matw_{1} \\
B \matu_{0} + \matw_{0}
\end{bmatrix} \in \hilspace^{T}
\end{align*}
Now, we can rewrite $\matx_T$ as  $\matx_T = G_T \,\matz_{[T]}$, so that
\begin{align}
\Sigma_{1;T} := \Exp[\matx_{T}\otimes \matx_T] = G_{T}  \Exp[\matz_{[T]}\otimes \matz_{[T]} ] G_T^{\herm} \label{eq:ExpX_eq}
\end{align}
Given a general linear operator $X: \calU \to \calV$, define $\diag_T(X): \calU^T \to \calV^T$ as the block diagonal operator with $T$ copies of $X$ on its diagonal. Observe that if it holds that, for some psd $\tLambda: \hilspace \to \hilspace$, that $\Exp[\matz_{[T]}\otimes \matz_{[T]}]  \preceq \diag_T(\tLambda)$, then by \Cref{eq:ExpX_eq},
\begin{align*}
\Sigma_{1} &= \lim_{T \to \infty}  G_{T}  \Exp[\matz_{[T]}\otimes \matz_{[T]} ] G_T^{\herm} \\
&\preceq \lim_{T \to \infty}  G_{T}\diag_T(\tLambda) G_{T} \\
&= \lim_{T \to \infty} \sum_{t=0}^{T-1} \Acltwo^{t} \tLambda \left(\Acltwo^\herm\right)^t = \dlyap{(A + B K_2)^\herm}{\tLambda}.
\end{align*}

Hence, it remains to bound $\Exp[\matz_{[T]} \otimes \matz_{[T]}] $.  Let us introduce the shorthand $\matu_{[T]} \defeq (\matu_{T-1}, \matu_{T-2},\dots,\matu_{0})$, and similarly for $\matw_{[T]}$ and $\matx_{[T]}$. Then, using the definition of $\matz_{[T]}$ and the fact that $\matu_{t} = (K_1 - K_2)\matx_t$,
\begin{align}
\Exp[\matz_{[T]} \otimes \matz_{[T]}] & = \Exp[(\diag_T(B) \matu_{[T]} + \matw_{[T]})^{\otimes 2}  ] \nn\\
&= \Exp[(\diag_T(B (K_1 - K_2)) \matx_{[T]} + \matw_{[T]})^{\otimes 2}] \nn\\
&\preceq 2\diag_T(B (K_1 - K_2))\cdot \Exp[ \matx_{[T]} \otimes \matx_{[T]}] \cdot \diag_T(B (K_1 - K_2))^{\herm}  + 2\Exp[\matw_{[T]} \otimes \matw_{[T]}]\nn\\
&= 2\diag_T(B (K_1 - K_2))\cdot \Exp[ \matx_{[T]} \otimes \matx_{[T]}] \cdot \diag_T(B (K_1 - K_2))^{\herm}  + 2\diag_T(\Lambda), \label{eq:zTbound_lastline}
\end{align}
where in the last line, $\Exp[\matw_{[T]} \otimes \matw_{[T]} ] = \diag(\Lambda)$ follows since $\matw_{[T]} = (\matw_{T-1},\dots,\matw_0)$, and $\matw_t \iidsim \calN(0,\Lambda)$ for $t \ge 0$. To bound $\Exp[ \matx_{[T]} \otimes \matx_{[T]} ]$, let us set $\matw_{-1} \defeq 0$ for simplicity, and $\matw_{[T],-1} \defeq (\matw_{T-2},\dots,\matw_{0},\matw_{-1})$, which corresponds to a shift of $\matw_{[T]}$. Finally, introduce the block Toeplitz operator:
\begin{align*}
\Toep_T: \hilspace^T \to \hilspace^T, \text{ with blocks } \Toep[i,j] = \Aclone^{j-i} \cdot \I_{j \ge i}.
\end{align*}
Then, we have the identity $\matx_{[T]} = \Toep_T \matw_{[T],-1},$
which implies that
\begin{align}
\Exp \matx_{[T]} \otimes \matx_{[T]} = \Toep_T \Exp \left[\matw_{[T],-1} \otimes \matw_{[T],-1}\right] \Toep_T^{\herm}\preceq  \Toep_T \cdot \diag_T(\Lambda) \cdot \Toep_T^{\herm}, \label{eq:matx_t_bound}
\end{align}
where we use that $\matw_{-1} = 0$ and $\matw_{t} \iidsim \calN(0,\Lambda)$ for $t \ge 0$. To conclude, let us decompose $\Toep_T$ into single-band operators via $Y_n: \hilspace^T \to \hilspace^T$ for $n \in \{0,1,\dots,T-1\}$, via:
\begin{align} \label{eq:Toep_decomp}
\Toep_T = \sum_{n=1}^{T}Y_n, \text{ where } Y_n: \hilspace^T \to \hilspace^T \text{ has blocks } Y_n[i,j] = \I_{ j = i + n - 1} \cdot A_1^{n - 1}.
\end{align}
Hence, continuing from \Cref{eq:matx_t_bound}, and applying the substitution in \Cref{eq:Toep_decomp}, by \Cref{lemma:outer_product_bound} we have that
\begin{align*}
\Exp \matx_{[T]}^{\otimes 2} &\preceq  \Toep_T \cdot \diag_T(\Lambda) \cdot \Toep_T^{\herm} \tag{\Cref{eq:matx_t_bound}}\\
&=  \left(\sum_{n=1}^T Y_n\right)\cdot \diag_T(\Lambda) \cdot \left(\sum_{n=1}^T Y_n\right)^{\herm} \tag{\Cref{eq:Toep_decomp}}\\
&\preceq 2 \sum_{n=1}^T n^2 \cdot  Y_n \diag_T(\Lambda)Y_n^{\herm} \tag{\Cref{lemma:outer_product_bound}}
\end{align*}
A simple computation reveals that $X_n \defeq Y_n \diag_T(\Lambda)Y_n^{\herm}$ is block diagonal with $i$-th block given by,
\[
X_n[i,i] = \I_{i \ge n} \Aclone^{n-1} \Lambda \left( \Aclone^{\herm} \right)^{n-1}.
\]
\jcpnote{I'm not totally confident that the indices for expressions involving Toeplitz operators are 100\% correct.}

Thus, $\left(\sum_{n=1}^T n^2 \cdot  Y_n \diag_T(\Lambda)Y_n^{\herm}\right)$ is block diagonal with $i$-th block given by
\begin{align*}
\sum_{n = 1}^{T- i + 1} n^2 \cdot \Aclone^{n-1} \Lambda \Aclone^{(n-1)\herm} &\preceq \sum_{n \ge 0} (n+1)^2 \cdot  \Aclone^{n}\Lambda \Aclone^{n \herm} \\
&= \sum_{n \ge 0} (n+1)^2 \cdot (A + BK_1)^{n}\Lambda (A + B K_1)^{n \herm} = \dlyapm{\Aclone}{\Lambda}{2}
\end{align*}
Hence, $\Exp \matx_{[T]} \otimes \matx_{[T]} \preceq 2\diag_T\left(\dlyapm{\Aclone}{\Lambda}{2}
\right)$. Combining with \Cref{eq:zTbound_lastline} gives
\begin{align*}
\Exp[\matz_{[T]} \otimes \matz_{[T]}] &\preceq 2\diag_T( B (K_1 - K_2))\cdot \Exp[ \matx_{[T]} \otimes \matx_{[T]} ] \cdot \diag_T( B (K_1 - K_2))^{\herm}  + 2\diag_T(\Lambda), \\
&\preceq 4\diag_T(B (K_1 - K_2))\cdot \diag_T\left(\dlyapm{\Aclone}{\Lambda}{2}
\right) \cdot \diag_T(B (K_1 - K_2))^{\herm}  + 2\diag_T(\Lambda)\\
&=4\diag_T\left(B (K_1 - K_2) \dlyapm{\Aclone}{\Lambda}{2} (K_1 - K_2)^{\herm} B^{\herm}\right)  + 2\diag_T(\Lambda)\\
&=\diag_T\left(4 B (K_1 - K_2) \dlyapm{\Aclone}{\Lambda}{2}(K_1 - K_2)^{\herm} B^{\herm} + 2\Lambda\right).
\end{align*}
This concludes the proof.

\end{proof}

\begin{lemma}\label{lemma:outer_product_bound} Let $Z \succeq 0$ and $Y_1,\dots,Y_T$ be bounded linear operators on a Hilbert space $\hilbx$. Then,
\begin{align*}
\left(\sum_{t=1}^{T}Y_t\right) Z \left(\sum_{t=1}^{T}Y_t\right)^{\herm} \preceq 2 \sum_{t=1}^T t^2 \, Y_t Z Y_t^{\herm}.
\end{align*}
\end{lemma}
\begin{proof} Let $\matx$ be any vector in $\hilbx$, then
\[
\innerHx{\matx}{\left(\sum_{t=1}^{T}Y_t\right) Z \left(\sum_{t=1}^{T}Y_t\right)^{\herm} \matx} = \innerHx{Z^{1/2} \left(\sum_{t=1}^{T}Y_t\right)^{\herm} \matx}{Z^{1/2} \left(\sum_{t=1}^{T}Y_t\right)^{\herm} \matx} = \normHx{\sum_{t=1}^T Z^{1/2} \left(\sum_{t=1}^{T}Y_t\right)^{\herm} \matx}^2
\]
Therefore it suffices to show that, for any  $\matx_1,\dots,\matx_T \in \hilbx$, $\normHx{\sum_{t=1}^T \matx_t}^2 \le 2\sum_{t=1}^T t^2 \cdot \normHx{\matx_t}^2$. We argue by Cauchy Schwartz,
\begin{align*}
\normHx{\sum_{t=1}^T \matx_t}^2 = \normHx{\sum_{t=1}^T \frac{1}{t} \cdot t \cdot \matx_t}^2 \le \left(\sum_{t=1}^T \frac{1}{t^2}\right) \cdot \sum_{t=1}^T \normHx{t \cdot \matx_t}^2.
\end{align*}
Since $\sum_{t=1}^T \frac{1}{t^2} = \frac{\pi^2}{6} \le 2$, the bound follows.
\end{proof}

\newpage
 \begin{corollary}
\label{corollary:change_of_controller}
Let $K_1$ be a stabilizing controller for the instance $\Ast, \Bst$. Then, for any stabilizing $K_2$,
\[
\dlyap{(\Ast + \Bst K_1)^\herm}{\expcovone} \preceq \calC_K \cdot \dlyap{(\Ast + \Bst K_2)^\herm}{\expcovone}
\]
for
\[
\calC_K \defeq 2\left(1 + \frac{36 \opnorm{K_2 - K_1}^2}{\sigma^2_\matu} \opnorm{\expcovone} \opnorm{P_1}^3 \log(2 \opnorm{P_1})^2 \right)
\]
where $P_1  \defeq \PinftyK{K_1}{\Ast}{\Bst}$
\end{corollary}

\begin{proof}
We apply \Cref{prop:HS_change_of_measure} to get that,
\[
\dlyap{(\Ast + \Bst K_1)^\herm}{\expcovone} \preceq \dlyap{(\Ast + \Bst K_2)^\herm}{\tLambda}
\]
for $$\tLambda = 2 \expcovone + 4 \Bst (K_1 - K_2)\dlyapm{(\Ast + \Bst K_1)^\herm}{\expcovone}{2}(K_1 - K_2)^{\herm} \Bst^{\herm}
.$$
Since $\expcovone = \dlyap{(\Ast + \Bst \Kinit)^\herm}{\uvar \Bst \Bst^\herm  + \covw} \succeq \sigma^2_\matu \Bst\Bst^\herm$, then letting $\Delta_{\mathsf{op}} = \opnorm{K_2 - K_1}$ we have that
\begin{equation}
\label{eq:tlambda_upper_bound}
\tLambda \preceq 2\left(1 + \frac{2 \Delta_{\mathsf{op}}^2}{\sigma^2_\matu} \opnorm{\dlyapm{(\Ast + \Bst K_1)^\herm}{\expcovone}{2}}\right)  \expcovone.
\end{equation}
Lastly, by \Cref{lemma:dlyapm_bound}, for any $n \geq 0$, we can upper bound $\opnorm{\dlyapm{(\Ast + \Bst K_1)^\herm}{\expcovone}{2}}$ by
\[
n^2 \opnorm{\dlyap{(\Ast + \Bst K_1)^\herm}{\expcovone}} + (n^2 + 2n + 2) \opnorm{\expcovone} \opnorm{P_1}^4 \exp\left( -n \opnorm{P_1}^{-1}\right).
\]
Using \Cref{lemma:dlyap_psd_ineq}, this last expression is in turn upper bounded by,
\[
n^2 \opnorm{\expcovone} \opnorm{P_1} + (n^2 + 2n + 2) \opnorm{\expcovone} \opnorm{P_1}^4 \exp\left( -n \opnorm{P_1}^{-1}\right)
\]
Setting $n = n_0 \defeq 3 \opnorm{P_1} \log(2 \opnorm{P_1})$, we get that
\[
(n_0^2 + 2n_0 + 2) \opnorm{\expcovone} \opnorm{P_1}^4 \exp\left( -n_0 \opnorm{P_1}^{-1}\right) \leq n_0^2 \opnorm{\expcovone} \opnorm{P_1}\]
this expression is less than. Therefore,
\[
\opnorm{\dlyapm{(\Ast + \Bst K_1)^\herm}{\expcovone}{2}} \leq 18 \opnorm{\expcovone} \opnorm{P_1}^3 \log(2 \opnorm{P_1})^2 \
\]
Plugging this upper bound into \cref{eq:tlambda_upper_bound} finishes the proof.
\end{proof}

\jcpnote{technically $n$ needs to be an integer?}
